# Supplementary material for: Probing the Structure of Deuteron at Very Short Distances
Source: arXiv:2108.11502 source file (2021-08-25)
Supplement: Supplementary file 1 [file appendixK.tex]

\chapter{Relativistic Wave Function - {\color{red}Hamiltonian}}
\label{App. RWF - Hamiltonian}

% As it follows from the above discussion the calculation of the cross-section on the light-front requires the knowledge of { LF} wave function of the nucleus.  
% At the  present the  most reliable approaches for calculation of { LF} wave function exist for two-nucleon systems.

Relativistic quantum mechanics requires that the description of the system by two observers must be equivalent if their reference frames { (RF)} are related by any Poincaré transformation, i.e. their RFs differ by either a rotation in space, a relative velocity, a translation in space-time or any combination of them \footnote{Lorentz transformations plus translations.}. This is to say that the  { WF}
of the system as described on each RF must be related by a unitary transformation \footnote{This assure  expectation values to be invariant.} associated with the Poincare transformation relating the { RFs} \cite{Foldy1960}.

From the set of operators that generate this kind of transformations infinitesimally, there are two  independent quadratic combinations that commute with all the generators, commonly referred as Casimir operators.
These are, {$M^2=P^{2}$} and {$W^2$}, the squares of the mass and spin operators respectively.

The 
Pauli-Lubanski pseudo-vector, { $W_\mu = {1 \over 2}\epsilon_{\mu \nu \alpha \beta} P^\nu J^{\alpha \beta}$}, is the relativistically covariant form of angular momentum. It is customary to define the angular momentum in the center of mass frame, for massive particles, which is the only case considered here, 
{ $(0,\mathbf{J_{cm}})=\Lambda_{cm}^{-1}(P_0)^\mu_{\ \nu} W^\nu/M$}, where {$\Lambda_{cm}^{-1}(P_0)^\mu_{\ \nu} \ $}  represents a  Lorentz transformation from  a reference frame 
where the particle has  momentum {$p_0$} to its rest frame.

The dynamics for two interacting particles on the { LF} is given by the Hamiltonian,
\begin{align}
H = H_{\text{free}}+V =	p_{1}^- + p_{2}^- + V = {p_{1 \ \textbf{T}}^2 + m_1^2 \over p_1^+} + {p_{2 \ \textbf{T}}^2 + m_2^2 \over p_2^+} + V  
\label{Hamiltonian} 
\end{align}   
which has the structure of a two-body non-relativistic Hamiltonian,
where the kinetic term is given by
\begin{equation}
H_{\text{free}}=\sum_i {p^2_{i \bf{T}} \over 2m_i  } + E_0
\end{equation}
with, {$2m_i=p^+_i$}, {$E_0=m_i^2/p_i^+$}, and {$V$} represents the interaction.  The wave function satisfies  the Schroedinger-like equation, 
\begin{align}
-i{\partial \over \partial x^+} \Psi = H \Psi 
\label{Schroedinger eq}
\end{align}   
where the evolution is in light-cone time, {$\tau=x^+$}. 
Within { LF} dynamics it is possible to factorize  the { WF} into external variables and  internal  ones, {$\Psi^d= \Psi^d_{\text{cm}}(\textbf{P}_{\text{cm}}) \Psi^d(\textbf{k}_\text{rel})$}, where the c.m. term {($ {\bf{P}}_{\text{cm}}=\bf{p}_1 + \bf{p}_2$)} describes the motion of deuteron as a whole, i.e. it does not play a role in the 2-body interaction.

The LF internal relative momentum  of the  particles is more conveniently given by the three-vector {$\textbf{k}$},
\begin{align}
& k^{\textbf{T}}=(1-\alpha)p_1^{\textbf{T}} - \alpha \ p_2^{\textbf{T}} \nonumber \\ 
&k^3= (\alpha - {1 \over 2})M_{12} -{m_1^2 - m_2^2 \over 2 M_{12}}  \label{relative k}
\end{align}  
which is helpful to express the { WF} in rotational invariant form. In Eq.(\ref{relative k})  {$M_{12} = \epsilon_1 + \epsilon_2 = (m_1^2 + \textbf{k}^2)^{1/2} + (m_2^2 + \textbf{k}^2)^{1/2} $}, and {$\alpha = { (\epsilon_1 + k_3) / M_{12} } $}.
The { LF-WF} for deuteron in these variables takes the form,
\begin{align}\label{deuteron wf}
\Psi^{LF}_d(\alpha, \textbf{k}_{\textbf{T}}) = R_{M1}^\dagger(\alpha, \textbf{k}_{\textbf{T}})  R_{M2}^\dagger(1-\alpha, -\textbf{k}_{\textbf{T}}) {\psi_d(\textbf{k}) \left( \textbf{k}^2_\textbf{T}+m^2\right)^{1/4} \over 2[(\alpha(1-\alpha))] ^{3/4} } 
\end{align}   
where the operator {$R_M$}, is the Melosh rotation Eq.(\ref{Melosh 2-component}),
%{ (Eq.(\ref{Melosh rot}))}, 
which relates the nucleons { LF} spinors 
%total spin { $\Sigma_{LF}$} 
to their instant-form (canonical spinors) 
%$\mathbf{J}_{cm}$ 
in the center of momentum frame of the pair
\begin{align}\label{Melosh rot}
R_{M} (\alpha , \textbf{p}_\text{T})= { p^+ + m - i \sigma \cdot (\textbf{n} \times \textbf{p}_\text{T} ) \over \sqrt{(p^+ + m)^2 + \textbf{p}^2_\text{T} }  }= { p^+ + m - i \textbf{n} \cdot (\textbf{p}_\text{T} \times \sigma ) \over \sqrt{(p^+ + m)^2 + \textbf{p}^2_\text{T} }  }   \rightarrow {  p^+ + m +   ( \textbf{p}_\text{T} \cdot \sigma_\text{T} ) ( {\sigma} \cdot \textbf{n} ) \over \sqrt{(p^+ + m)^2 + \textbf{p}^2_\text{T} }  }  
\end{align}  
with $ \textbf{n}$ is a unit vector perpendicular to the LF surface.

The Melosh transformation allows us to combine the spin  and  orbital angular momentum of individual nucleons in the usual additive manner,
\begin{align}\label{angular mom sum}
\Sigma_{LF} = R_{M1}^\dagger R_{M2}^\dagger \textbf{J}_{\text{cm}}^{ \text{total}} R_{M1} R_{M2} =\textbf{ L}(\textbf{k}) + \textbf{s}_1 + \textbf{s}_2  
\end{align}  
where the 
%LF constituent 
spin operators for the nucleons, {$\textbf{s}_i= R_{Mi}^\dagger \ \textbf{j}_{i,\text{cm}}  R_{Mi}$}, are 
%given by the constituent nucleon spins  
defined in the rest frame of the pair, 
	$(0,\mathbf{j}_{i, \text{cm}})=\Lambda_{\textbf{P}_{\text{cm}}}^{-1}(\textbf{p}_{i})^\mu_{\ \nu} W^\nu/M$.
It follows that the familiar Clebsh-Gordon decomposition can be used to give a description in terms of angular momentum eigenfunctions, {$\Sigma_{LF}$}, {$\Sigma_{LF}^3$}, where the latter is the angular momentum projection along  $k^3$ direction.

The relativistic description must be rotational  invariant, this is needed to guaranty the proper commutation relations among the Poincaré generators. 

For this we require that the Hamiltonian must commute with the spin operator, {$ \left[ H , \Sigma_{LF} \right] =0 $} \footnote{Whereby, the { WF}  admits a partial wave decomposition.}. 
This imposes restrictions over the Poincaré generators, known as the angular condition. Some generators, in this case of rotations, must contain the interaction
%This requirement is 
%needed 
in order 
to guaranty the proper commutation relations among them.
It can be fulfilled if the potential {($V$)} in the Hamiltonian is only function of euclidean  products of 3-vectors (sufficient condition), since these are invariant under spatial rotations \cite{Bakker1979}. For the 2-body case it means scalar products  among the internal variables,   {$\textbf{k}, \ \textbf{L}, \ \textbf{s}_1, \ \textbf{s}_2$}. Under this conditions, the { LF-WF} can be expressed, in the center of mass frame of the two nucleons, through the  { S} and { D} partial waves of deuteron  \cite{FS1991}, 
{\footnotesize$$ \psi_d(\textbf{k})^{s_d}= \bar{u}(\textbf{p}_1) {1 \over \epsilon^{1/2}}  \left[ \gamma^{s_d}  \left(  u(k) - {1\over \sqrt{2}}w(k)  \right)  + {(p_1 - p_2 )^{s_d} \over k^2}  \left( (\epsilon -m ) u(k)  + (2\epsilon + m )  \right) {1\over \sqrt{2}}w(k)  \right] u(\textbf{p}_2) $$ }
where, { $\epsilon=\sqrt{m^2+k^2}$} and both nucleon masses are approximated by {$m=(m_p+m_n)/2$}.
