# Supplementary material for: Probing the Structure of Deuteron at Very Short Distances
Source: arXiv:2108.11502 source file (2021-08-25)
Supplement: Supplementary file 2 [file appendixL.tex]

\chapter{Angular Condition}    \label{Angular Condition}

{\color{Green}
The EM current operator represents the generator of transition amplitudes for the conserved EM charge. It appears (conventionally) in the Lagrangian contracted with the field that mediates the interaction, i.e. the EM gauge field (minimal coupling, $A^\mu J_\mu$). 
%Thus, it must transform like a Lorentz four-vector to guarantee the 
Invariance of the action requires that this contraction transform like a scalar. {\color{Purple} 
	The most restrictive way to achieve this is forcing $J_\mu$ to behave like a four-vector 
\footnote{{\color{blue} In the general case we may not know how to solve some of the interactions, e.g., in QCD.  Yet, we still can guarantee the correct transformations properties of the current by using Gauge invariance constrains (Ward-Takahashi relations).}}. 
} 
This is conveniently  expressed by the following commutation relation with the Lorentz generators, $M_{\nu \rho}$ (rotations and boosts), which every four-vector must obey {\color{red} [Polyzou1991, Keister1994]}\cite{Karmanov:1995},
\begin{equation}\label{EM current transf}
\left[ J_\mu,M_{\nu \rho}\right]= i(g_{\mu\nu}J_\rho - g_{\mu\rho}J_\nu)
\end{equation}
Within a field theoretical approach, the generators of Poincare transformations are found from the Lagrangian via the energy-momentum tensor (Noether theorem). If  interactions are included, {\it i.e.} when the Lagrangian include terms combining more than two fields (e.g. $A^\mu J_\mu$), 
{\color{Purple} the dynamical evolution of the system can be study by writing the theory in Hamiltonian form. This is done by choosing the ``time-direction'' in order to perform the necessary Legendre transformation that relates the Lagrangian and Hamiltonian descriptions. This procedure breaks the (trivial) invariance (embedded in the Lagrangian) by introducing a special coordinate (time). Covariance is then achieved by guarantying that quantities transform like the components of Lorentz structures (four-vectors, tensors, ...), forcing that 
	}
some of the Lorentz generators,  $M_{\nu \rho}$, 
must include the interactions \footnote{In general one must consider the non homogeneous Lorentz group (Poincare group). Then, some of the generators, $M_{\nu \rho}, \ P_\mu$, must include the interactions. For example, in the Point Form of Hamiltonian dynamics the interaction is packed into $P_\mu$. In this work we restrict ourselves to the Instant and Light Front forms of Hamiltonian dynamics, in which case the interactions are packed into $M_{\mu\nu}$.}. This implies that if any of the Lorentz generators includes information about the coupling between fields, then the EM current on the right hand side of Eq.(\ref{EM current transf}) must contain the interaction as well.

%{\color{blue}
For the case of Light Front quantization formulations  it has been stressed  {\color{red}[Frankfurt, Strikman, Mankiewicz, Sawicki 1990]} that there is a non-trivial difficulty associated to the angular momentum operator (AMO) containing the interaction, i.e. to perform a general rotation on an interacting system one must have already solved the dynamical problem because the AMO depends on it. 
In contrast, the AMO within a Canonical (Instant form) formulation is trivial (kinematical). Thus angular distributions for example can be generated from any particular solution by applying the standard (kinematical)  generators of rotations. For on-shell scattering process (and approximately for small missing-energy {\color{red} (inelasticity)} reactions) the interaction (``potential'', i.e. green-function-kernel) must depend only on rotational invariant quantities, e.g. scalar products of 3-vectors ($\boldsymbol{p}\cdot \boldsymbol{k}$) {\color{red}[FSMS1990]}.

For off-shell scattering process the situation is more complicated. 
% The purpose of the present work is to address this issue. 
%However, this is in fact deceiving. 
In this case the canonical (instant form) formulation shows its deficiencies.   The instant form boosts are dynamical, thus the solution to the scattering on bound particles with ``large'' relative momentum must be done for each particular value of the momentum, as it turns out this is more difficult to deal with than the rotational problem. 

%Since, the best way to investigate/test our knowledge in the quantum realm is through EM probes. On this regard, 
Moreover, looking to rhs of Eq.(\ref{EM current transf}) we can see that, because the matrix of the instant form metric is diagonal there is no  component of the (canonical) current with vanishing commutator.  On the other hand, choosing $\mu=+$ we see that  for the LF component $J^+$ the commutator do vanishes, which had make it earned the name of ``good current''. 

{\color{red} A frequent criticism to LF approaches is the use of (simple sum) one-body currents ... }

%}
